# Supplementary material for: Classification and mapping of low-statured 'shrubland' cover types in post-agricultural landscapes of the US Northeast
Source: arXiv:2205.05047 source file (2022-12-21)
Supplement: Supplementary file 1 [file supplementary_materials.pdf]

# Supplementary Materials

## Table of contents

**Supplementary Materials 1: LiDAR Data Sets** 2

**Supplementary Materials 2: LT-GEE Parameters** 4

**Supplementary Materials 3: Component Model Accuracies** 5

Random Forest (ranger) . . . . . . . . . . 5

Stochastic GBM (LightGBM) . . . . . . . . . . 6

Neural Net (keras) . . . . . . . . . . 7

**References** 8

## Supplementary Materials 1: LiDAR Data Sets

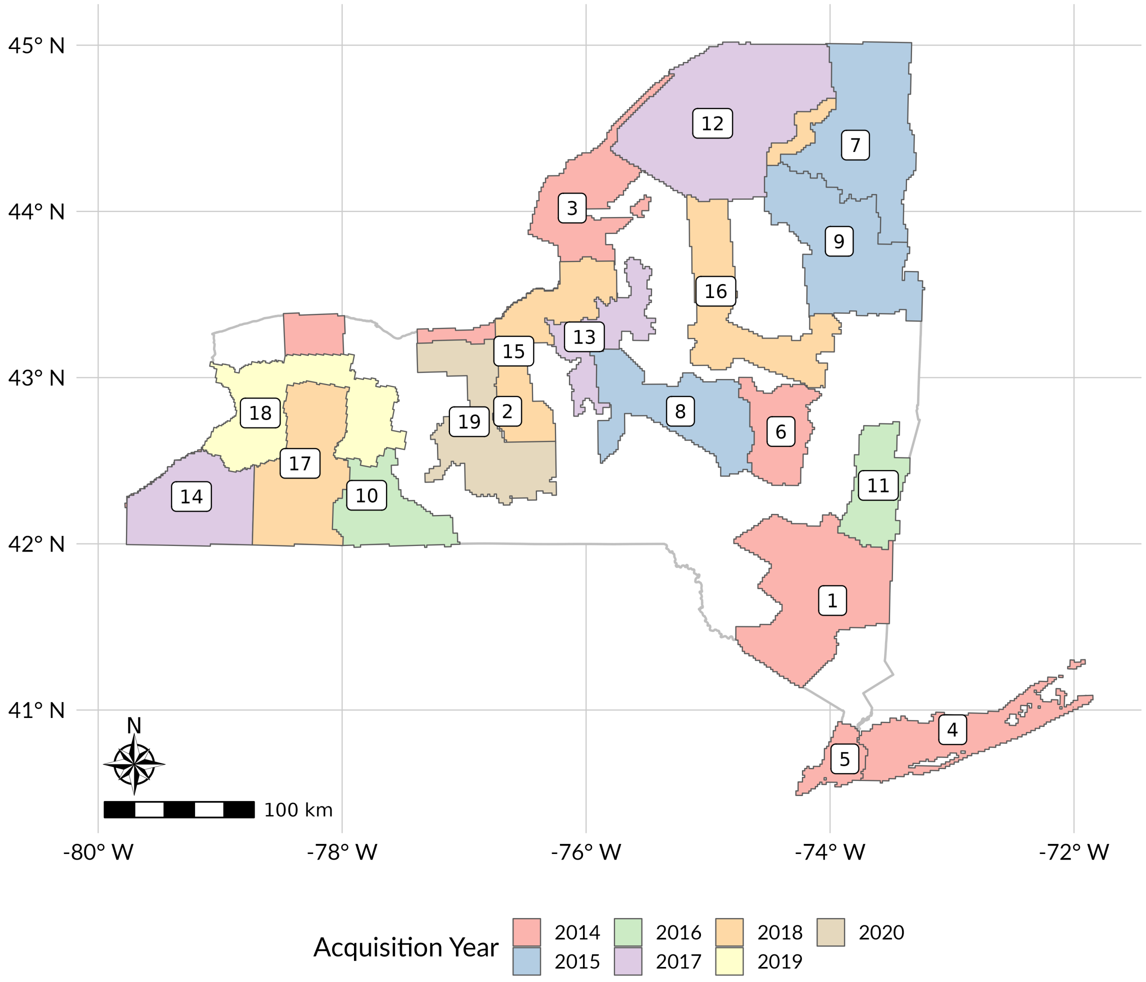


Figure 1: Boundaries for all LiDAR coverages used in this project, colored by year of data acquisition. Numbers on each coverage represent the "index" value of that coverage in table Supplementary Materials 1.

Table 1: Lidar boundaries. “Index” numbers reflect identifier numbers as used in Supplementary Materials Figure 1. Region names reflect the naming conventions used by the NYSGPO; this often, but not always, reflects included counties. Area values are approximate and in square kilometers. Density values are in points per square meter (ppm).

| Index | Region Name | Acquisition Year | Area | Density | Citation |
|---|---|---|---|---|---|
| 1 | 3 County | 2014 | 7,370 | 2.04 | United States Geological Survey (2015a) |
| 2 | Great Gully | 2014 | 720 | 2.16 | Axis GeoSpatial, LLC (2014) |
| 3 | Great Lakes | 2014 | 5,780 | 2.04 | United States Geological Survey (2015c) |
| 4 | Long Island | 2014 | 3,170 | 2.04 | Woolpert, Inc (2014a) |
| 5 | NYC | 2014 | 790 | 2.04 | Woolpert, Inc (2014b) |
| 6 | Schoharie | 2014 | 2,500 | 2.04 | United States Geological Survey (2015b) |
| 7 | Clinton, Essex & Franklin | 2015 | 1,110 | 2.04 | Quantum Spatial (2016) |
| 8 | Madison & Otsego | 2015 | 4,780 | 2.18 | Axis GeoSpatial, LLC (2016a) |
| 9 | Warren, Washington & Essex | 2015 | 6,280 | 3.24 | Atlantic Inc (2015) |
| 10 | Allegany & Steuben | 2016 | 3,410 | 2.04 | New York Office of Information Technology Services (2016) |
| 11 | Columbia & Rensselaer | 2016 | 2,600 | 2.60 | Axis GeoSpatial, LLC (2016b) |
| 12 | Franklin & St. Lawrence | 2017 | 9,880 | 2.04 | Quantum Spatial (2017b) |
| 13 | Oneida Subbasin | 2017 | 2,550 | 2.04 | Quantum Spatial (2017a) |
| 14 | Southwest | 2017 | 4,460 | 2.04 | New York Office of Information Technology Services (2017) |
| 15 | Cayuga & Oswego | 2018 | 4,450 | 2.04 | New York Office of Information Technology Services (2018a) |
| 16 | Fulton, Saratoga, Herkimer & Franklin | 2018 | 5,010 | 1.98 | Quantum Spatial (2018) |
| 17 | Southwest (B) | 2018 | 5,660 | 2.04 | New York Office of Information Technology Services (2018b) |
| 18 | Erie, Genesee & Livingston | 2019 | 5,670 | 2.04 | New York Office of Information Technology Services (2019) |
| 19 | Central Finger Lakes | 2020 | 5,040 | 2.04 | New York Office of Information Technology Services (2021) |

## Supplementary Materials 2: LT-GEE Parameters

Table 2: Landtrendr Google Earth Engine (LT-GEE) segmentation parameters for 10 Landsat-derived predictors (Kennedy et al. 2018).

| Parameters | Annual Reflectance (NBR, TC*) | Disturbance (YOD, MAG) |
|---|---|---|
| maxSegments | 5 | 10 |
| spikeThreshold | 0.5 | 0.9 |
| vertexCountOvershoot | 3 | 3 |
| preventOneYearRecovery | true | true |
| recoveryThreshold | 0.25 | 0.75 |
| pvalThreshold | 0.05 | 0.05 |
| bestModelProportion | 0.75 | 0.75 |
| minObservationsNeeded | 6 | 6 |

Table 3: Disturbance predictor (YOD, MAG) parameters in LT-GEE.

| Parameter | Value | Operator |
|---|---|---|
| Delta | Loss | |
| Sort | Most recent | |
| Year | 1985-Target year | |
| Magnitude | 50 | Greater than |
| Duration | 4 | Less than |
| Pre-disturbance spectral value | 300 | Greater than |
| Minimum mapping unit | 7 | |

## Supplementary Materials 3: Component Model Accuracies

These tables replicate Table 3 from the manuscript for each of the component models. Metrics reflect equations and definitions from Section 2.4.

### Random Forest (ranger)

Table 4: Model accuracy metrics for the random forest model with predictions classified using various thresholds, calculated using both the balanced test set and the LiDAR patchwork surface. AUC for the LiDAR patchwork was calculated using a random sample of 1,000,000 pixels, while all other metrics used all predicted pixels. Thresholds were selected using a separate validation set, using values chosen to maximize the Youden J statistic ("Youden optimal") or to target a certain minimum specificity ("% specificity").

| | Threshold | Sensitivity | Specificity | Precision | F1 |
|---|---|---|---|---|---|
| **Test set (AUC: 0.843)** | | | | | |
| Youden optimal | 0.519 | 0.767 | 0.752 | 0.754 | 0.760 |
| 90% specificity | 0.602 | 0.537 | 0.900 | 0.841 | 0.655 |
| 95% specificity | 0.648 | 0.379 | 0.951 | 0.885 | 0.531 |
| 99% specificity | 0.704 | 0.135 | 0.990 | 0.930 | 0.236 |
| **LiDAR patchwork (AUC: 0.844)** | | | | | |
| Youden optimal | 0.519 | 0.767 | 0.750 | 0.075 | 0.137 |
| 90% specificity | 0.602 | 0.533 | 0.898 | 0.122 | 0.199 |
| 95% specificity | 0.648 | 0.376 | 0.950 | 0.164 | 0.228 |
| 99% specificity | 0.704 | 0.135 | 0.990 | 0.253 | 0.176 |

## Stochastic GBM (LightGBM)

Table 5: Model accuracy metrics for the gradient boosting machine model with predictions classified using various thresholds, calculated using both the balanced test set and the LiDAR patchwork surface. AUC for the LiDAR patchwork was calculated using a random sample of 1,000,000 pixels, while all other metrics used all predicted pixels. Thresholds were selected using a separate validation set, using values chosen to maximize the Youden J statistic ("Youden optimal") or to target a certain minimum specificity ("% specificity").

| | Threshold | Sensitivity | Specificity | Precision | F1 |
|---|---|---|---|---|---|
| **Test set (AUC: 0.889)** | | | | | |
| Youden optimal | 0.498 | 0.837 | 0.776 | 0.787 | 0.811 |
| 90% specificity | 0.699 | 0.644 | 0.900 | 0.864 | 0.738 |
| 95% specificity | 0.787 | 0.485 | 0.949 | 0.905 | 0.632 |
| 99% specificity | 0.889 | 0.208 | 0.990 | 0.955 | 0.342 |
| **LiDAR patchwork (AUC: 0.890)** | | | | | |
| Youden optimal | 0.519 | 0.838 | 0.773 | 0.089 | 0.161 |
| 90% specificity | 0.602 | 0.642 | 0.899 | 0.144 | 0.235 |
| 95% specificity | 0.648 | 0.482 | 0.949 | 0.199 | 0.282 |
| 99% specificity | 0.704 | 0.207 | 0.990 | 0.349 | 0.260 |

## Neural Net (keras)

Table 6: Model accuracy metrics for the neural net model with predictions classified using various thresholds, calculated using both the balanced test set and the LiDAR patchwork surface. AUC for the LiDAR patchwork was calculated using a random sample of 1,000,000 pixels, while all other metrics used all predicted pixels. Thresholds were selected using a separate validation set, using values chosen to maximize the Youden J statistic ("Youden optimal") or to target a certain minimum specificity ("% specificity").

| | Threshold | Sensitivity | Specificity | Precision | F1 |
|---|---|---|---|---|---|
| **Test set (AUC: 0.883)** | | | | | |
| Youden optimal | 0.494 | 0.830 | 0.774 | 0.784 | 0.806 |
| 90% specificity | 0.704 | 0.618 | 0.901 | 0.861 | 0.720 |
| 95% specificity | 0.791 | 0.441 | 0.950 | 0.899 | 0.592 |
| 99% specificity | 0.886 | 0.185 | 0.987 | 0.942 | 0.309 |
| **LiDAR patchwork (AUC: 0.901)** | | | | | |
| Youden optimal | 0.519 | 0.838 | 0.773 | 0.089 | 0.161 |
| 90% specificity | 0.602 | 0.642 | 0.899 | 0.144 | 0.235 |
| 95% specificity | 0.648 | 0.482 | 0.949 | 0.199 | 0.282 |
| 99% specificity | 0.704 | 0.207 | 0.990 | 0.349 | 0.260 |

## References

Atlantic Inc. 2015. "NY_WarrenWashingtonEssex_Spring2015." ftp://ftp.gis.ny.gov/elevation/LIDAR/.

Axis GeoSpatial, LLC. 2014. "13367 Great Gully LiDAR." ftp://ftp.gis.ny.gov/elevation/LIDAR/.

———. 2016a. "Axis GeoSpatial, LLC New York Tiled LiDAR." ftp://ftp.gis.ny.gov/elevation/LIDAR/.

———. 2016b. "New York Office of Information Technology Services Classified LiDAR Tiles." ftp://ftp.gis.ny.gov/elevation/LIDAR/.

New York Office of Information Technology Services. 2016. "Allegany and Steuben Counties, New York Lidar; Overall Project Metadata." ftp://ftp.gis.ny.gov/elevation/LIDAR/.

———. 2017. "Southwest 17 - Spring, New York Lidar; Classified Point Cloud." ftp://ftp.gis.ny.gov/elevation/LIDAR/.

———. 2018a. "LIDAR Collection (QL2) for Cayuga County and Most of Oswego County, New York Lidar; Classified Point Cloud." ftp://ftp.gis.ny.gov/elevation/LIDAR/.

———. 2018b. "Southwest 17-b - Fall, New York Lidar; Classified Point Cloud." ftp://ftp.gis.ny.gov/elevation/LIDAR/.

———. 2019. "LIDAR Collection (QL2) for Erie, Genesee, and Livingston Counties New York Lidar; Classified Point Cloud." ftp://ftp.gis.ny.gov/elevation/LIDAR/.

———. 2021. "Lidar Collection (QL2) of All or Part of Schuyler, Seneca, Steuben, Tompkins, Wayne and Yates Counties, NY Lidar; Classified Point Cloud." ftp://ftp.gis.ny.gov/elevation/LIDAR/.

Quantum Spatial. 2016. "Clinton-Essex-Lake Champlain New York 2015 LiDAR USGS Contract: G10PC00026 Task Order Number: G10PC00026 and G14PD000943 (Modification) NY_ClintonEssex_2015." ftp://ftp.gis.ny.gov/elevation/LIDAR/.

Quantum Spatial, Inc. 2017a. "New York FEMA 2016 QL2 LiDAR - Central Zone AOI; Classified Point Cloud." ftp://ftp.gis.ny.gov/elevation/LIDAR/.

———. 2017b. "New York FEMA 2016 QL2 LiDAR - East Zone AOI; Classified Point Cloud." ftp://ftp.gis.ny.gov/elevation/LIDAR/.

———. 2018. "Lidar Collection (QL2) of All or Part of Schuyler, Seneca, Steuben, Tompkins, Wayne and Yates Counties, NY Lidar; Classified Point Cloud." ftp://ftp.gis.ny.gov/elevation/LIDAR/.

United States Geological Survey. 2015a. "LAS." ftp://ftp.gis.ny.gov/elevation/LIDAR/.

———. 2015b. "LAS." ftp://ftp.gis.ny.gov/elevation/LIDAR/.

———. 2015c. "LAS Extents." ftp://ftp.gis.ny.gov/elevation/LIDAR/.

Woolpert, Inc. 2014a. "USGS Long Island New York Sandy Lidar Classified LAS 1.2." ftp://ftp.gis.ny.gov/elevation/LIDAR/.

———. 2014b. "USGS New York CMGP Sandy Lidar." ftp://ftp.gis.ny.gov/elevation/LIDAR/.
